# Supplementary material for: A Learning Framework for Distribution-Based Game-Theoretic Solution Concepts
Source: arXiv:1903.08322 source file (2019-06-16)
Supplement: Supplementary file 1 [file appendix.tex]

\appendix
\section{Omitted Proofs}
\begin{proof}[Proof of Corollary~\ref{corr:conjuncts}]
	While the first claim follows immediately from definition of uniform convergence, and the third is a direct consequence of Boole-Frechet inequalities.
	\begin{itemize}
		\item[Part 1 (Simultaneous Constraints)] is a direct corollary of Theorem \ref{thm:upperbound}; if $m \geq \underset{i}{\max} m^{\UC}_i(\epsilon, \delta)$, then $$\forall i \in [k], g \in \G_{|T}, s \in \Sol: \underset{T \sim {\cal D}^m}{\Pr}[ \lvert {L_i}_T (g, s) - {L_i}_{\cal D} (g, s) \rvert > \epsilon] < \delta$$
		
		\item[Part 2 (Separable Conjunctions)] By definition graph dimension, $\Sd_G(\probleminstance_1)$ is the size of the largest shattered set in $\tup{\cal X_\probleminstance, \cal Y_\probleminstance, \G_\probleminstance, \Sol_1, \lambda_1}$, and $\Sd_G(\probleminstance_2)$ for $\tup{\cal X_\probleminstance, \cal Y_\probleminstance, \G_\probleminstance, \Sol_2, \lambda_2}$. Without loss of generality, let us assume $\Sd_G(\probleminstance_1) \geq \Sd_G(\probleminstance_2)$.
		Also, empirical loss is $$L_T(g, s) = L_T(g, \tup{s_1, s_2}) = \frac{1}{|T|} \sum\limits_{(x_j,g(x_j)) \in T} \lambda_1(x_j,g,s_1) \wedge \lambda_2(x_j,g,s_2)$$
		Define, for any given $s_2 \in \Sol_2$, define a $\probleminstance_{1|s_2} = \tup{\cal X_\probleminstance, \cal Y_\probleminstance, \G_\probleminstance, \Sol_1, \lambda_{1|s_2}}$, where 
\[\lambda_{1|s_2}(x,g,s_1) = \left\{
  \begin{array}{lr}
    0 & : \text{if }\lambda_2(x,g,s_2)=0 \\
    \lambda_1(x,g,s_1) & : \text{otherwise.}
  \end{array}
\right.
\]
		Observe that the empirical loss and statistical loss for $\lambda_{1|s_2}$ is equivalent to the empirical loss and statistical loss of the conjunction of $\lambda_1$ and $lambda_2$, respectively. Also, observe that any set shattered in $\probleminstance_{1|s_2}$ will also be shattered $\probleminstance_{1}$, and has sample complexity $m^{\UC}(\epsilon, \delta) \in \tilde{\cal O}(\Sd_G(\probleminstance_1))$.
		
		\item[Part 3 (Bounded Disjunctions)] If $m \geq \underset{i}{\max} m^{\UC}_i(\epsilon/k, \delta)$, then we know that for all $i$:
		$$\underset{T \sim {\cal D}^m}{\Pr}[ \underset{x \sim \cal D}{Pr}[\lambda_{i}(x,g,s)] < \frac{\epsilon}{k} ] < \delta$$
		Since, by union bound, $\Pr[\bigvee_{i=1}^k \lambda_i(x,g,s)] \leq \sum_{i=0}^k \underset{x \sim \cal D}{Pr}[\lambda_{i^*}(x,g,s)]$, therefore we have
		$$\underset{T \sim {\cal D}^m}{\Pr}[ \underset{x \sim \cal D}{\Pr}[\bigvee_{i=1}^k \lambda_i(x,g,s)] < \epsilon ] < \delta$$
		And for constant $k$, $m^{\PAC}_i(\epsilon/k, \delta) \in O(m^{\PAC}_i(\epsilon, \delta))$, hence $m^{\PAC}(\epsilon, \delta) \in \tilde{\cal O}( \underset{i \in [k]}{\max} m^{\PAC}(\probleminstance_i))$.
	\end{itemize}
	\end{proof}
\begin{proof}[Proof of Corollary~\ref{corr:pac-solving-ERM-bounds}]
\begin{itemize}
\item[Part 1 (Worst-case Agnostic PAC Solving)] Let $\cal A_m : (\cal X \times \cal Y)^m \rightarrow \Sol$ be an ERM Solver such that for any sample of $m \geq m^{\UC}(\eps, \delta)$ points $T = \langle (x_i, y_i) \rangle_{i=1}^m$, outputs a solution $\cal A (T) \in \Sol$ that minimizes $\underset{g \in \G|_{T}}{\max} L_T(g, \cal A (T) )$. 

Let $s^* \in \Sol$ be a solution such that it minimizes $\underset{g \in \G|_{T}}{\max} L_{\cal D}(g, s^* )$. By definition of $\cal A (T)$, we know $$\underset{g \in \G|_{T}}{\max} L_T(g, \cal A (T) ) \leq \underset{g \in \G|_{T}}{\max} L_T(g, s^* ).$$ And similarly we know, for statistical loss, $$\underset{g \in \G|_{T}}{\max} L_{\cal D}(g, s^* ) \leq \underset{g \in \G|_{T}}{\max} L_{\cal D}(g, \cal A (T) ).$$

For size of sample $m  \geq m^{\UC}(\eps /2, \delta)$, we know by Theorem \ref{thm:upperbound}, that with likelihood $\geq \delta$, 
$$\underset{g \in \G|_{T}}{\max} L_{\cal D}(g, \cal A (T) ) 	.$$
And,
$$.$$

For any $g_0 \in \G_{|T}$, by Theorem \ref{thm:upperbound}, $L_{\cal D}(g, \cal A (T) ) \in (L_T(g, \cal A (T) ) - \eps, L_T(g, \cal A (T) ) + \eps)$.

Let the $s^* \in \Sol$ be the solution that minimizes $\underset{g \in \G|_{T}}{\max} L_{\cal D}(g, s^*)$. For $g_0$, $L_{T}(g, s^* ) \in (L_{\cal D}(g, s^* ) - \eps, L_{\cal D}(g, s^* ) + \eps)$.

If $m \geq m^{\UC}(\eps, \delta)$, then we know $$\forall g \in \G_{|T}, s \in \Sol: \underset{T \sim {\cal D}^m}{\Pr}[ \lvert {L}_T (g, s) - {L}_{\cal D} (g, s) \rvert > \epsilon] < \delta$$

\item[Part 2 (Bayesian Agnostic PAC Solving)] Let $\cal A_m : (\cal X \times \cal Y)^m \rightarrow \Sol$ be an ERM Solver such that for any sample of $m$ points $T = \langle (x_i, y_i) \rangle_{i=1}^m$, outputs a solution $s^{*} \in \Sol$ that minimizes $\underset{g^\prime \sim \ddot{\cal D}}{E} [L_D(g^\prime, s)| g^\prime \in \G|_{T}]$ (with or without the knowledge of the prior $\ddot{\cal D}$).
\end{itemize}
\end{proof}
